# Supplementary material for: Reviewing Labels: Label Graph Network with Top-k Prediction Set for Relation Extraction
Source: arXiv:2212.14270 source file (2022-12-29)
Supplement: Supplementary file 1 [file appendix.tex]

\section{Datasets}\label{dataset}

We use the following three datasets in our research:

\begin{itemize}
    \item \textbf{TACRED.} TACRED is the most widely used relation extraction dataset. It contains 42 relations, including "No Relation". The relations in TACRED are imbalanced. 
    \item \textbf{TACRED-Revisit.} This dataset is the modified version of TACRED, with the same statistical information as TACRED, and is relabeled on the test set only.
    \item \textbf{SemEval2010.} SemEval2010 contains 10 different relation names, including "No Relation".
\end{itemize}

\begin{table}[h]
\begin{tabular}{l|l|l|l|l}
\hline
Dataset   & \#Train & \#Dev  & \#Test & \#Class \\ \hline
TACRED    & 68,124  & 22,613 & 15,509 & 42      \\
TACRED-Revisit    & 68,124  & 22,613 & 15,509 & 42      \\
SemEval   & 8,000   & -      & 2,712  & 10      \\\hline
\end{tabular}
\caption{Statistics of different RE datasets used in our experiments. SemEval2010 does not have the validation set. \#classes contain the `No Relation' instances.}
\label{data}
\end{table}

\section{Parameter Searching}\label{param}

\begin{table}[h]
\centering
\setlength{\tabcolsep}{1.3mm}
\begin{tabular}{c|c}
\toprule[1.5pt]
\textbf{Parameters}            & \textbf{Ranges}                              \\ \hline
\textbf{Max Epochs}            & \{5,10,15,20\}                               \\ \hline
\textbf{Peak Learning Rate}    & \{1e-6, 5e-6, 1e-5, 5e-5, 1e-4, 5e-4\} \\ \hline
\textbf{Batch Size}            & \{4, 8, 16, 24, 32\}                         \\ \hline
\textbf{Warm-up Ratio}         & \{0.05, 0.1, 0.15, 0.2\}                     \\ \hline
\textbf{Sequence Length}       & \{128, 192, 256, 320\}                       \\ \hline
\textbf{$\tau$}   & \{0.01, 0.05, 0.1\}                          \\ \hline
\textbf{$\alpha$} & \{0.8, 0.85, 0.9, 0.95\}                     \\ \hline
\textit{k}                     & \{2, 4, 6, 8, 10\}                           \\ \bottomrule[1.5pt]
\end{tabular}
\caption{Hyperparameter ranges searched for fine-tuning TACRED, TACRED-Revisit and SemEval2010.}
\end{table}

\section{Other Explorations}\label{app_1}
As a pioneering work of using the \textit{Top-k} prediction set, we also conduct some explorations. Under the assumption that we already have the \textit{Top-k} prediction set for each example, there are several simple and straightforward ways to utilize this information. 

\noindent\textbf{Label Smoothing.} 
The idea of label smoothing was first proposed by Inception-v2 \cite{DBLP:conf/icml/IoffeS15}. It changes the one-hot label vector into a soft label. Intuitively, label smoothing restraints the logit value for the correct class to be closer to the logit values for other classes. We use label smoothing to force the model to pay attention to the labels in the \textit{Top-k} prediction set. Specifically, we modify the one-hot label as the soft label, and the loss $\mathcal{L}$ is computed as follows:
\begin{equation}
    \mathcal{L} = \gamma\mathcal{L}^{CE}(i) + \frac{1 - \gamma}{k}\sum_{j \in \textit{s(Top-k)}}\mathcal{L}^{CE}(j).\label{softlabel}
\end{equation}
Where $\gamma$ = 0.9 in our experiment. By using the soft label. Equation \ref{softlabel} makes the model pay attention to labels in the \textit{Top-k} prediction set.

\noindent\textbf{Prompt.}
Also, we can write a prompt and give some clues to the model. A prompt contains the \textit{Top-k} prediction set and some natural language, which may be helpful for the model to understand the available information existing in the \textit{Top-k} prediction set. Specifically, for a given input text and its \textit{Top-k} prediction set \textit{s(Top-k)}, we add a prompt $P$ after the input text, and $P$ is: Choose a relation from \textit{s(Top-k)} for the $e_1$ and the $e_2$. Where $e_1$ and $e_2$ denote the head entity and tail entity. To avoid the model simply selecting the first label in the \textit{s(Top-k)} as output, we randomly shuffle the orders of labels in \textit{s(Top-k)}.

\noindent\textbf{Generation Objective Extension.}
In this setting, we design a model that uses BART and force it to generate the ground truth first, and then the model also needs to generate labels in the \textit{Top-k} prediction set one by one. With this generation objective, we hope the encoder-decoder architecture could learn the semantic connection from the generation objectives, and use the \textit{Top-k} prediction set effectively.

Note that the above three strategies are only applied to the baseline models, such as RoBERTa-large and BART-large. To help readers better understand our model design, we take a training sentence from TACRED as an example and show the detailed settings in Table \ref{example}.

\section{The Performances Using Other Backbone Networks}\label{othermodel}

\begin{table}[h]
\centering
\setlength{\tabcolsep}{1.3mm}
\begin{tabular}{cccc}
\toprule[1.5pt]
\multicolumn{1}{c|}{}                    & \multicolumn{1}{c|}{\textbf{TACRED}} & \multicolumn{1}{c|}{\textbf{TACRED-Rev}} & \textbf{SemEval} \\ \hline
\multicolumn{4}{l}{\textit{\textbf{BERT-base}}}                                                                                               \\ \hline
\multicolumn{1}{c|}{\textbf{Base Model}} & \multicolumn{1}{c|}{71.2}            & \multicolumn{1}{c|}{79.0}                & 89.0             \\
\multicolumn{1}{c|}{\textbf{LG-topk w/o DM}}         & \multicolumn{1}{c|}{72.0(+0.8)}      & \multicolumn{1}{c|}{79.6(+0.6)}          & 89.3(+0.3)       \\
\multicolumn{1}{c|}{\textbf{LG-topk}}        & \multicolumn{1}{c|}{72.5(+1.3)}      & \multicolumn{1}{c|}{80.2(+1.2)}          & 89.6(+0.6)       \\ \hline
\multicolumn{4}{l}{\textit{\textbf{BERT-large}}}                                                                                              \\ \hline
\multicolumn{1}{c|}{\textbf{Base Model}} & \multicolumn{1}{c|}{72.7}            & \multicolumn{1}{c|}{80.9}                & 89.3             \\
\multicolumn{1}{c|}{\textbf{LG-topk w/o DM}}         & \multicolumn{1}{c|}{73.6(+0.9)}      & \multicolumn{1}{c|}{81.6(+0.7)}          & 89.5(+0.2)       \\
\multicolumn{1}{c|}{\textbf{LG-topk}}        & \multicolumn{1}{c|}{74.2(+1.5)}      & \multicolumn{1}{c|}{82.1(+1.2)}          & 89.8(+0.5)       \\ \bottomrule[1.5pt]
\end{tabular}
\caption{Performances using different backbone networks.}
\label{other_backbone}
\end{table}

We also report the performances using different backbone networks, e.g., BERT-base \footnote{https://huggingface.co/bert-base-uncased} and BERT-large \footnote{https://huggingface.co/bert-large-uncased}.. From Table \ref{other_backbone} we can observe that our model obtains consistent improvements compared to corresponding Base Models. The above results show that LG-topk works well with various backbone networks on three RE datasets.

\begin{table*}[t]
\centering
\setlength{\tabcolsep}{1.3mm}
\begin{tabular}{l|l|c}
\toprule[1.5pt]
                        & \multicolumn{1}{c|}{\textbf{Input}}                                                                                                                                                                                                                                                                    & \textbf{Output}                                                                                                                                                        \\ \hline
\textbf{Base Model}     & \begin{tabular}[c]{@{}l@{}}@ Lindsay Hayes @ , a national \# specialist \# \\ prison suicide prevention who wrote the report...\end{tabular}                                                                                                                                                           & One-hot Label                                                                                                                                                          \\ \hline
\textbf{Base Model(P)}  & \begin{tabular}[c]{@{}l@{}}@ Lindsay Hayes @ , a national \# specialist \# \\ prison suicide prevention who wrote the report...\\ Choose a relation from \{per:title, org:founded, \\ org:shareholders, no\_relation, per:city\_of\_birth, \\ per:age\} for Lindsay Hayes and specialist.\end{tabular} & One-hot Label                                                                                                                                                          \\ \hline
\textbf{Base Model(LS)} & \begin{tabular}[c]{@{}l@{}}@ Lindsay Hayes @ , a national \# specialist \# \\ prison suicide prevention who wrote the report...\end{tabular}                                                                                                                                                           & Soft Label                                                                                                                                                             \\ \hline
\textbf{BART}           & \begin{tabular}[c]{@{}l@{}}@ Lindsay Hayes @ , a national \# specialist \# \\ prison suicide prevention who wrote the report...\end{tabular}                                                                                                                                                           & per:title                                                                                                                                                              \\ \hline
\textbf{BART(GOE)}      & \begin{tabular}[c]{@{}l@{}}@ Lindsay Hayes @ , a national \# specialist \# \\ prison suicide prevention who wrote the report...\end{tabular}                                                                                                                                                           & \multicolumn{1}{l}{\begin{tabular}[c]{@{}l@{}}per:title $|$ per:title $|$ org:founded $|$ \\ org:shareholders $|$ no\_relation $|$ \\ per:city\_of\_birth $|$ per:age\end{tabular}} \\ \bottomrule[1.5pt]
\end{tabular}
\caption{An example from the TACRED dataset. For \textbf{BART(GOE)}, we use the first relation name of the output sequence as the prediction.}
\label{example}
\end{table*}
